# Supplementary material for: Entropy Measures of Human Communication Dynamics
Source: arXiv:1801.04528 source file (2018-01-14)
Supplement: Supplementary file 1 [file supplement.tex]

\documentclass[fleqn,10pt]{wlscirep}

\begin{document}

\end{document}
